# Supplementary material for: The First Flight of the Marshall Grazing Incidence X-ray Spectrometer (MaGIXS)
Source: arXiv:2212.00665 source file (2022-12-07)
Supplement: Supplementary file 1 [file appendix.tex]

\appendix

If needed.
